# Supplementary material for: One-Dimensional Edge Contact to Encapsulated MoS2 with a Superconductor
Source: arXiv:2101.06194 source file (2021-01-15)
Supplement: Supplementary file 1 [file Supplementary.tex]

\setcounter{figure}{0}
\setcounter{page}{1}
\setcounter{equation}{0}
\setcounter{section}{0}

\section{Sample Fabrication}

Both van der Waals heterostructures studied in this work were assembled with a dry transfer technique using a polyethylene terephthalate (PET) stamp [citations]. Flakes of hBN and MoS$_2$ were mechanically exfoliated onto Si/SiO$_2$ substrates, lifted with the PET stamp at 60 $^{\circ}$C, and deposited on a clean Si/SiO$_2$ (300 nm oxide layer) chip at 130 $^{\circ}$C. PET residue was removed from the top of the heterostructure and from the surrounding substrate by immersion in dichloromethane for one hour at 70 $^{\circ}$C.

Prior to the patterning of the contacts, an alignment grid and array of bonding pads and leads (each 5/45 nm Cr/Au) were lithographically defined and thermally evaporated onto both substrates. The one-dimensional interface between the MoS$_2$ and the MoRe was prepared via electron-beam lithography, reactive ion etching (RIE), and sputtering. Standard lithographic techniques were used to define the locations of the superconducting contacts, with a PMMA resist and a cold isopropyl alcohol / de-ionized water (3:1) develop step. Josepshon junctions were placed so as to avoid bubbles trapped between the layers of the heterostructure.

Reactive ion etching was used to reveal the MoS$_2$ edge from within the heterostructure. The etching recipe consisted of three steps, all carried out using a Trion Technology Phantom II RIE system with a process pressure of 10$^{-1}$ Torr. First, a ten second CHF$_3$ / O$_2$ (10:1 flow rate ratio) step to remove any PMMA reside from the top surface of the heterostructure. This was followed by a ten second SF$_6$ process to etch through the top hBN. Finally, a ten second CF$_4$ step was used to etch the MoS$_2$ in the contact region. While a CF$_4$ etch is a typical process for MoS$_2$, SF$_6$ may itself be sufficient \cite{Jain2019}. In order to limit the device’s exposure to atmosphere, and so the formation of MoO$_x$ along the interface, the device was not removed from the system and imaged between these steps.

The devices were held under vacuum following the RIE process. The second sample was treated with an Ar+ sputtering process [details] before metal deposition to refresh the contact interface. Both received 100 nm of MoRe (50-50\% by weight) with process pressures ~ 10$^{-8}$ Torr. To minimize processing, the junctions were not etched after the deposition of MoRe, and so the flakes of MoS$_2$ continue beyond the boundaries of the junctions. This is visible in Figure 1, which details the final device geometries.

 Annealing** (200C overnight for N1, 350 overnight for N3; 10$^-6$ mbar; N1 destroyed with 300C Ar+H2 flow)

\section{Sample Annealing}
\label{section:anneal}

Figure \ref{fig:anneal} shows that the annealing processes cause the contact to become significantly worse. This is similar to Ref. (Jain), where the poor adhesion to hBN causes the metal to reflow away from the material. Additional explanations include (whatever Gleb suggests).

\begin{figure}
    \centering
    \includegraphics[width=\linewidth]{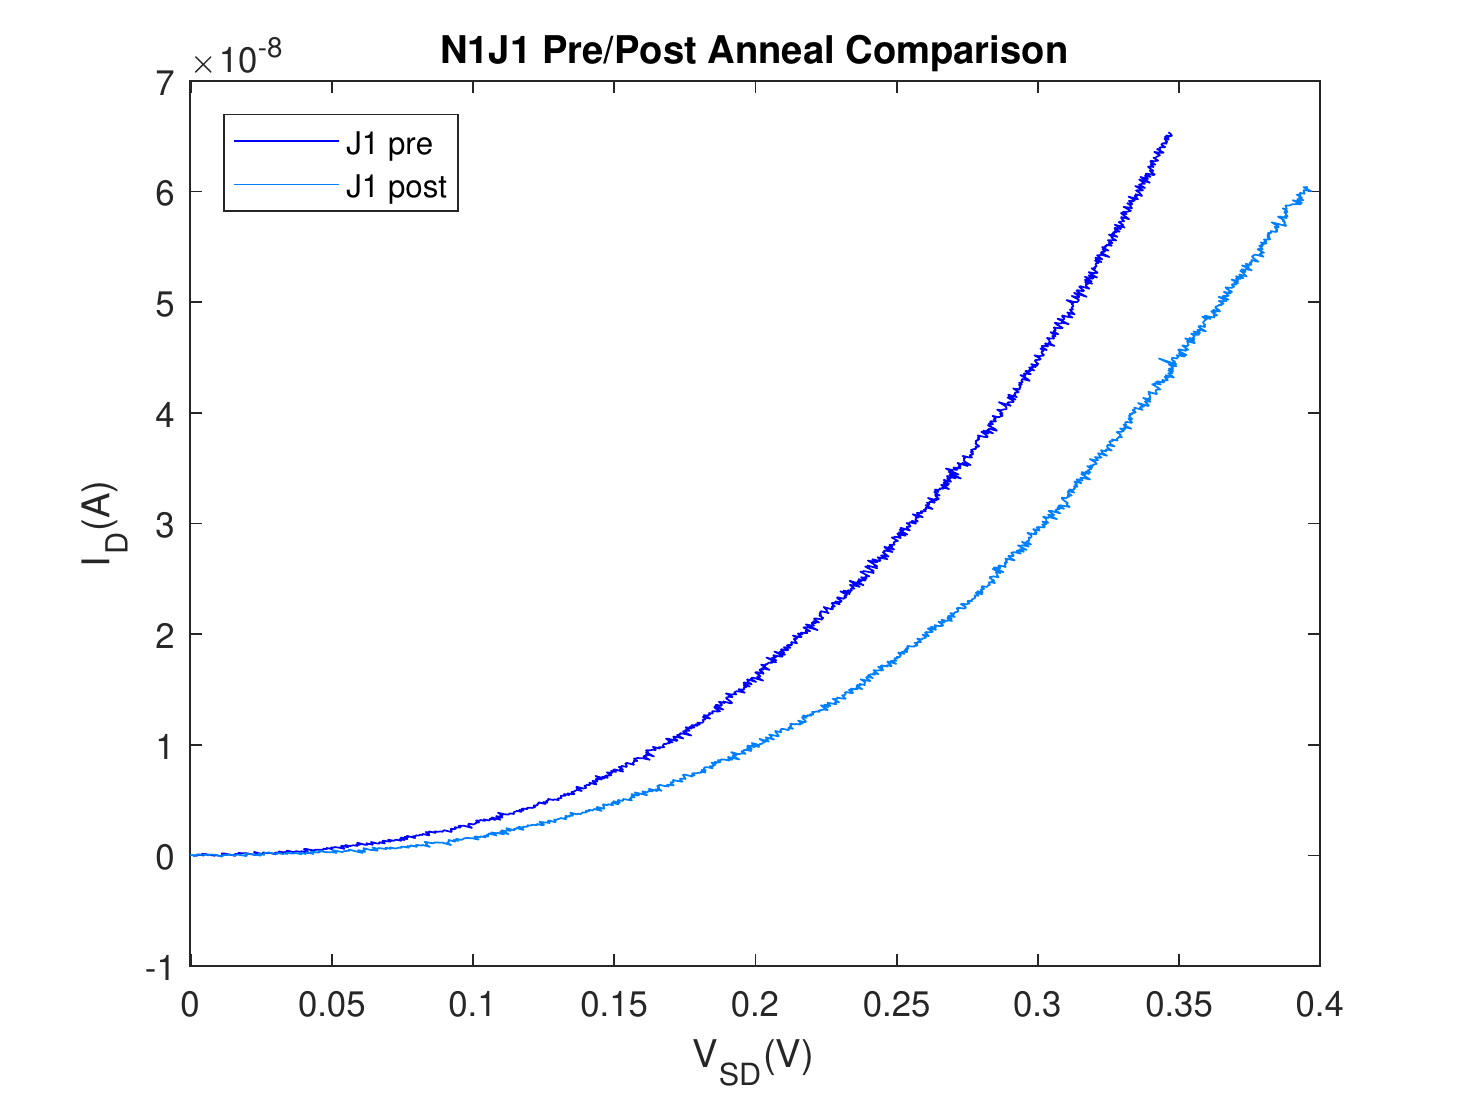}
    \caption{Newaz 1, J1, pre and post anneal comparison, $V_{BG}$=42 V.}
    \label{fig:anneal}
\end{figure}
